# Supplementary material for: Plug-and-Play Transformer Modules for Test-Time Adaptation
Source: arXiv:2401.04130 source file (2024-02-08)
Supplement: Supplementary file 1 [file supp_index.tex]

\begin{table*}[t]
\centering
\begin{tabularx}{\textwidth}{c X}
    \toprule
    Section & Supplementary Material Overview\\
    \cmidrule(lr){2-2} 
    \ref{sec:supp_SAR} & Sharpness-aware domain adaptation\\
    \ref{sec:supp_parameterefficiency} & Parameter efficiency\\
    \ref{sec:supp_PETmethods} & Details on different PET methods\\
    \ref{sec:supp_HP}  & Hyperparameters\\
    \ref{sec:supp_corruption}  & Details of dataset corruptions\\
    \bottomrule
\end{tabularx}
\end{table*}
